# Supplementary material for: A fully algebraic and robust two-level Schwarz method based on optimal local approximation spaces
Source: arXiv:2207.05559 ancillary file (2022-07-12)
Supplement: Supplementary file 1 [file Algebraic_Robust_Schwarz_AH_KS_22_supplement.pdf]

# SUPPLEMENTARY MATERIALS: A FULLY ALGEBRAIC AND ROBUST TWO-LEVEL SCHWARZ METHOD BASED ON OPTIMAL LOCAL APPROXIMATION SPACES

ALEXANDER HEINLEIN AND KATHRIN SMETANA

## SM1. Full proof of the bound of the condition number

To show an upper bound for the condition number, typically one tries to satisfy three assumptions: a stable decomposition, strengthened Cauchy-Schwarz inequalities, and local stability [SM3]. As motivated in section 4 the stable decomposition yields a lower bound on $a_\Omega(P_{AS}u,u)$ and invertibility of $\boldsymbol{P}_{AS}$; see also [SM3]. As the strengthened Cauchy-Schwarz inequalities and the local stability yield together an upper bound for $a_\Omega(P_{AS}u,u)$, satisfying these three assumptions results in an upper bound for the condition number.

As we use exact local solvers (5), we have

$$a_{\Omega_i'}(u_i,v_i) = a_\Omega(E_{\Omega_i'\to\Omega}u_i, E_{\Omega_i'\to\Omega}v_i) \quad \forall u_i, v_i \in V^0_{\Omega_i'}.$$

Therefore, the following assumption is satisfied with $\omega = 1$:

**Assumption SM1.1** (Local stability [SM3, Assumption 2.4])**.** *There existis $\omega > 0$, such that*

$$a_\Omega(E_{\Omega_i'\to\Omega}u_i, E_{\Omega_i'\to\Omega}u_i) \le \omega a_{\Omega_i'}(u_i,u_i), \quad u_i \in \operatorname{range}(\widetilde{P}_i) \subset V^0_{\Omega_i'}, 0 \le i \le M.$$

**Assumption SM1.2** (Strengthened Cauchy-Schwarz inequalities [SM3, Assumption 2.3])**.** *There exist constants $0 \le \epsilon_{ij} \le 1$, $1 \le i,j \le M$, such that*

$$|a_\Omega(E_{\Omega_i'\to\Omega}u_i, E_{\Omega_i'\to\Omega}u_j)| \le \epsilon_{ij} a_\Omega(E_{\Omega_i'\to\Omega}u_i, E_{\Omega_i'\to\Omega}u_i)^{1/2} a_\Omega(E_{\Omega_i'\to\Omega}u_j, E_{\Omega_i'\to\Omega}u_j)^{1/2},$$

*for $u_i \in V^0_{\Omega_i'}$ and $u_j \in V^0_{\Omega_j'}$. The spectral radius of the matrix $\epsilon$ with entries $\epsilon_{ij}$ is denoted by $\rho(\epsilon)$.*

Denoting by the constant $m$ an upper bound for the number of overlapping subdomains $\Omega_i'$ any point in $\Omega$ can belong to, we obtain $\rho(\epsilon) \le m$. Thanks to [SM3, Lemma 3.11] we then obtain

$$a_\Omega(P_{AS}u,u) \le (m+1) a_\Omega(u,u) \quad \forall u \in V^0_\Omega. \tag{SM1}$$

To obtain an upper bound for the condition number it thus remains to verify the following assumption.

**Assumption SM1.3** (Stable decomposition [SM3, Assumption 2.2])**.** *There exists a constant $C_0$, such that every $u \in V^0_\Omega$ admits a decomposition*

$$u = E_0u_0 + \sum_{i=1}^{M} E_{\Omega_i'\to\Omega}u_i \tag{SM2}$$

*such that*

$$\sum_{i=0}^{M} a_{\Omega_i'}(u_i,u_i) \le C_0^2 a_\Omega(u,u). \tag{SM3}$$

*Date*: July 12, 2022.

SM1.1. **Bound of the coarse level and local contributions.** To improve readability, we split the proof of Lemma 6.2 in two results stated in Lemmas SM1.4 and SM1.5 and their respective proofs. For the steps of the proof of Lemmas SM1.4 and SM1.5 see also [SM1, SM2].

**Lemma SM1.4** (Bound of the coarse level contribution). *Let $m_e$ denote the maximal number of edges $e$ in a subdomain $\Omega_i$. Then, we have*

$$|u_0|^2_{a,\Omega} \leq 2|u|^2_{a,\Omega} + 2m_e \sum_{i=1}^{M} \sum_{e\subset\partial\Omega_i} \left|E_{e\to\Omega_e}\left[(u-u_0)|_e\right]\right|^2_{a,\Omega_e}, \tag{SM4}$$

*where $E_{e\to\Omega_e}$ has been defined in the beginning of subsection 5.1.*

*Proof.* By exploiting the definition of $u_0$ in (40) and that the Galerkin approximation minimizes the energy norm among all functions in the respective FE space, we obtain

$$\begin{aligned} |u_0|^2_{a,\Omega} &= |H_{\Gamma\to\Omega}(u_0|_\Gamma)|^2_{a,\Omega} \leq 2|H_{\Gamma\to\Omega}\left[(u-u_0)|_\Gamma\right]|^2_{a,\Omega} + 2|H_{\Gamma\to\Omega}(u|_\Gamma)|^2_{a,\Omega} \\ &\leq 2|H_{\Gamma\to\Omega}\left[(u-u_0)|_\Gamma\right]|^2_{a,\Omega} + 2|u|^2_{a,\Omega}. \end{aligned} \tag{SM5}$$

To estimate the first term in (SM5), we introduce the operators $E_{\partial\Omega_i\to\Omega_i} : V_{\partial\Omega_i} \to V_{\Omega_i}$ and $E_{e\to\Omega_i} : V_e^0 \to V_{\Omega_i}$, which assign the coefficients of the FE functions on $\partial\Omega_i$ and $e$ to the corresponding FE basis functions in $\Omega_i$, respectively, and zero to all remaining coefficients. Using again the energy-minimizing property of the Galerkin approximation, we obtain

$$\begin{aligned} |H_{\Gamma\to\Omega}\left[(u-u_0)|_\Gamma\right]|^2_{a,\Omega} &\leq \sum_{i=1}^{M} |H_{\partial\Omega_i\to\Omega_i}\left[(u-u_0)|_{\partial\Omega_i}\right]|^2_{a,\Omega_i} \\ &\leq \sum_{i=1}^{M} |E_{\partial\Omega_i\to\Omega_i}\left[(u-u_0)|_{\partial\Omega_i}\right]|^2_{a,\Omega_i}. \end{aligned}$$

Thanks to the definition of $u_0$ in (40), the function $u-u_0$ is zero in all vertices of the coarse decomposition, which yields

$$\begin{aligned} \sum_{i=1}^{M} |E_{\partial\Omega_i\to\Omega_i}\left[(u-u_0)|_{\partial\Omega_i}\right]|^2_{a,\Omega_i} &\leq \sum_{i=1}^{M} \left| \sum_{e\subset\partial\Omega_i} E_{e\to\Omega_i}\left[(u-u_0)|_e\right] \right|^2_{a,\Omega_i} \\ &\leq m_e \sum_{i=1}^{M} \sum_{e\subset\partial\Omega_i} \left|E_{e\to\Omega_i}\left[(u-u_0)|_e\right]\right|^2_{a,\Omega_i} \\ &\leq m_e \sum_{i=1}^{M} \sum_{e\subset\partial\Omega_i} \left|E_{e\to\Omega_e}\left[(u-u_0)|_e\right]\right|^2_{a,\Omega_e}. \end{aligned}$$

□

**Lemma SM1.5** (Bound of the local contributions). *Let $u_i$ be defined as in* (41) *and let $m_e$ denote the maximal number of edges $e$ in a subdomain $\Omega_i$. Then, we have*

$$\sum_{i=1}^{M} |u_i|^2_{a,\Omega_i'} \leq 18|u|^2_{a,\Omega} + 15m_e \sum_{i=1}^{M} \sum_{e\subset\partial\Omega_i} \left|E_{e\to\Omega_e}\left[(u-u_0)|_e\right]\right|^2_{a,\Omega_e}, \tag{SM6}$$

*where $E_{e\to\Omega_e}$ has been defined in the beginning of subsection 5.1.*

*Proof.* As we use exact local solvers (5), the operator $E_{\Omega_i'\to\Omega}$ simply extends FE functions in $V^0_{\Omega_i'}$ by zero, and $\widetilde{\Omega}_i \subset \Omega_i'$, we have

$$\sum_{i=1}^{M} a_{\Omega_i'}(u_i,u_i) = \sum_{i=1}^{M} a_{\Omega}(E_{\Omega_i'\to\Omega}u_i, E_{\Omega_i'\to\Omega}u_i) = \sum_{i=1}^{M} a_{\widetilde{\Omega}_i}(u_i|_{\widetilde{\Omega}_i}, u_i|_{\widetilde{\Omega}_i}).$$

Recall to that end that the subdomains $\widetilde{\Omega}_i$ form an overlapping decomposition of the domain $\Omega$ with overlap $h$ and that $\{\theta_i\}_{i=1}^M$ denotes a corresponding partition of unity. Next, we introduce subdomains $\widehat{\Omega}_i := \Omega_i \setminus \left\{\cup_j \widetilde{\Omega}_j\right\}, j \neq i$ where $\Omega_i \cap \widetilde{\Omega}_i = \Omega_i$, $i = 1,\dots,M$, and note that we have

$$\widetilde{\Omega}_i = \widehat{\Omega}_i \ \dot\cup \ \left(\Omega_i \setminus \widehat{\Omega}_i\right) \ \dot\cup \ \left(\widetilde{\Omega}_i \setminus \Omega_i\right).$$

As a consequence, we obtain

$$|u_i|^2_{a,\widetilde{\Omega}_i} = |u_i|^2_{a,\widehat{\Omega}_i} + |u_i|^2_{a,\Omega_i\setminus\widehat{\Omega}_i} + |u_i|^2_{a,\widetilde{\Omega}_i\setminus\Omega_i}, \tag{SM7}$$

where here and henceforth in this proof we omit the restriction to the respective subdomains such as $|_{\widetilde{\Omega}_i}$ to improve readability. Next, we bound the three terms on the right-hand side of (SM7) separately. Thanks to the bound for the coarse level contribution in (SM4) and the definition of $u_i$ in (41), we obtain for the first term

$$\begin{aligned}\sum_{i=1}^{M} |u_i|^2_{a,\widehat{\Omega}_i} &\overset{(41)}{\leq} \sum_{i=1}^{M} |u-u_0|^2_{a,\Omega_i} \leq 2\sum_{i=1}^{M} |u|^2_{a,\Omega_i} + 2\sum_{i=1}^{M} |u_0|^2_{a,\Omega_i} \\ &\overset{(42)}{\leq} 6|u|^2_{a,\Omega} + 4m_e \sum_{i=1}^{M} \sum_{e\subset\partial\Omega_i} \left|E_{e\to\Omega_e}\left[(u-u_0)|_e\right]\right|^2_{a,\Omega_e},\end{aligned}$$

where we have used Lemma SM1.4. To estimate the second term on the right-hand side in (SM7), we introduce the functions $\psi_i := 1-\theta_i$, $i=1,\dots,M$ noting that we have $|\psi_i| \leq 1$. Similarly as for the first term we obtain

$$\begin{aligned}\sum_{i=1}^{M} |u_i|^2_{a,\Omega_i\setminus\widehat{\Omega}_i} &= \sum_{i=1}^{M} \left|I^h\big(\theta_i(u-u_0)\big)\right|^2_{a,\Omega_i\setminus\widehat{\Omega}_i} \\ &\leq \sum_{i=1}^{M} \Big(2|u-u_0|^2_{a,\Omega_i\setminus\widehat{\Omega}_i} + 2\left|I^h\big(\psi_i(u-u_0)\big)\right|^2_{a,\Omega_i\setminus\widehat{\Omega}_i}\Big) \\ &\leq 4|u|^2_{a,\Omega} + 4|u_0|^2_{a,\Omega} + 2\sum_{i=1}^{M} \left|I^h\big(\psi_i(u-u_0)\big)\right|^2_{a,\Omega_i\setminus\widehat{\Omega}_i}.\end{aligned}$$

To conclude the estimate we wish to estimate the last term by $2\sum_{i=1}^{M} |E_{\partial\Omega_i\to\Omega_i}(u-u_0)|^2_{a,\Omega_i\setminus\widehat{\Omega}_i}$, where $E_{\partial\Omega_i\to\Omega_i}$ has been introduced in the proof of Lemma SM1.4. As both $u$ and $u_0$ are FE functions, the values of the functions $I^h\big(\psi_i(u-u_0)\big)$ and $E_{\partial\Omega_i\to\Omega_i}(u-u_0)$ are purely determined by their values on $\partial\Omega_i$ and $\partial\widehat{\Omega}_i$. Thanks to the definition of $\theta_i$ and $\psi_i$, we have $I^h\big(\psi_i(u-u_0)\big)(x) < (u-u_0)(x) = E_{\partial\Omega_i\to\Omega_i}(u-u_0)(x)$ for all $x \in \partial\Omega_i$. As both $I^h\big(\psi_i(u-u_0)\big)$ and $E_{\partial\Omega_i\to\Omega_i}(u-u_0)$ are zero on $\partial\widehat{\Omega}_i$, we thus obtain $I^h\big(\psi_i(u-u_0)\big)(x) \leq E_{\partial\Omega_i\to\Omega_i}(u-u_0)(x)$ for all $x \in \Omega_i \setminus \widehat{\Omega}_i$. This allows us to continue with the estimate similarly as in the proof of

Lemma SM1.4:

$$\begin{aligned}\sum_{i=1}^{M} |u_i|^2_{a,\Omega_i\setminus\widehat{\Omega}_i} &\leq 4|u|^2_{a,\Omega} + 4|u_0|^2_{a,\Omega} + 2\sum_{i=1}^{M} |E_{\partial\Omega_i\to\Omega_i}\left[(u-u_0)|_{\partial\Omega_i}\right]|^2_{a,\Omega_i\setminus\widehat{\Omega}_i} \\ &= 4|u|^2_{a,\Omega} + 4|u_0|^2_{a,\Omega} + 2\sum_{i=1}^{M} |E_{\partial\Omega_i\to\Omega_i}\left[(u-u_0)|_{\partial\Omega_i}\right]|^2_{a,\Omega_i} \\ &\leq 4|u|^2_{a,\Omega} + 4|u_0|^2_{a,\Omega} + 2m_e\sum_{i=1}^{M}\sum_{e\subset\partial\Omega_i} |E_{e\to\Omega_e}\left[(u-u_0)|_e\right]|^2_{a,\Omega_e} \\ &\overset{(42)}{\leq} 12|u|^2_{a,\Omega} + 10m_e\sum_{i=1}^{M}\sum_{e\subset\partial\Omega_i} |E_{e\to\Omega_e}\left[(u-u_0)|_e\right]|^2_{a,\Omega_e}.\end{aligned}$$

To estimate the third term on the right-hand side of (SM7), we introduce the operator $E_{\partial\Omega_i\to\widetilde{\Omega}_i} : V_{\partial\Omega_i} \to V_{\widetilde{\Omega}_i}$, which assigns the coefficients of the FE functions on $\partial\Omega_i$ to the corresponding FE basis functions in $\widetilde{\Omega}_i$ and zero to all remaining coefficients. Using a similar argumentation as in the estimate of the second term, we obtain

$$\sum_{i=1}^{M} |u_i|^2_{a,\widetilde{\Omega}_i\setminus\Omega_i} = \sum_{i=1}^{M} |I^h\big(\theta_i(u-u_0)\big)|^2_{a,\widetilde{\Omega}_i\setminus\Omega_i} \leq \sum_{i=1}^{M} |E_{\partial\Omega_i\to\widetilde{\Omega}_i}(u-u_0)|^2_{a,\widetilde{\Omega}_i\setminus\Omega_i}.$$

Arguing completely analogous to the proof of Lemma SM1.4 yields

$$\sum_{i=1}^{M} |u_i|^2_{a,\widetilde{\Omega}_i\setminus\Omega_i} \leq m_e\sum_{i=1}^{M}\sum_{e\subset\partial\Omega_i} |E_{e\to\Omega_e}\left[(u-u_0)|_e\right]|^2_{a,\Omega_e}.$$

Adding up the bounds for the three terms in (SM7) yields the claim. □

## References

[SM1] A. Heinlein, A. Klawonn, J. Knepper, and O. Rheinbach, *Multiscale coarse spaces for overlapping Schwarz methods based on the ACMS space in 2D*, Electron. Trans. Numer. Anal., 48 (2018), pp. 156–182.

[SM2] A. Heinlein, A. Klawonn, J. Knepper, and O. Rheinbach, *Adaptive GDSW coarse spaces for overlapping Schwarz methods in three dimensions*, SIAM J. Sci. Comput., 41 (2019), pp. A3045–A3072.

[SM3] A. Toselli and O. Widlund, *Domain decomposition methods—algorithms and theory*, vol. 34 of Springer Series in Computational Mathematics, Springer-Verlag, Berlin, 2005.

Delft Institute of Applied Mathematics, Delft University of Technology, The Netherlands. a.heinlein@tudelft.nl

Department of Mathematical Sciences, Stevens Institute of Technology, 1 Castle Point Terrace, Hoboken, NJ 07030, United States of America. ksmetana@stevens.edu
